# Supplementary material for: LLM-Based Multi-Agent Systems are Scalable Graph Generative Models
Source: arXiv:2410.09824 source file (2025-01-06)
Supplement: Supplementary file 1 [file control.pdf]

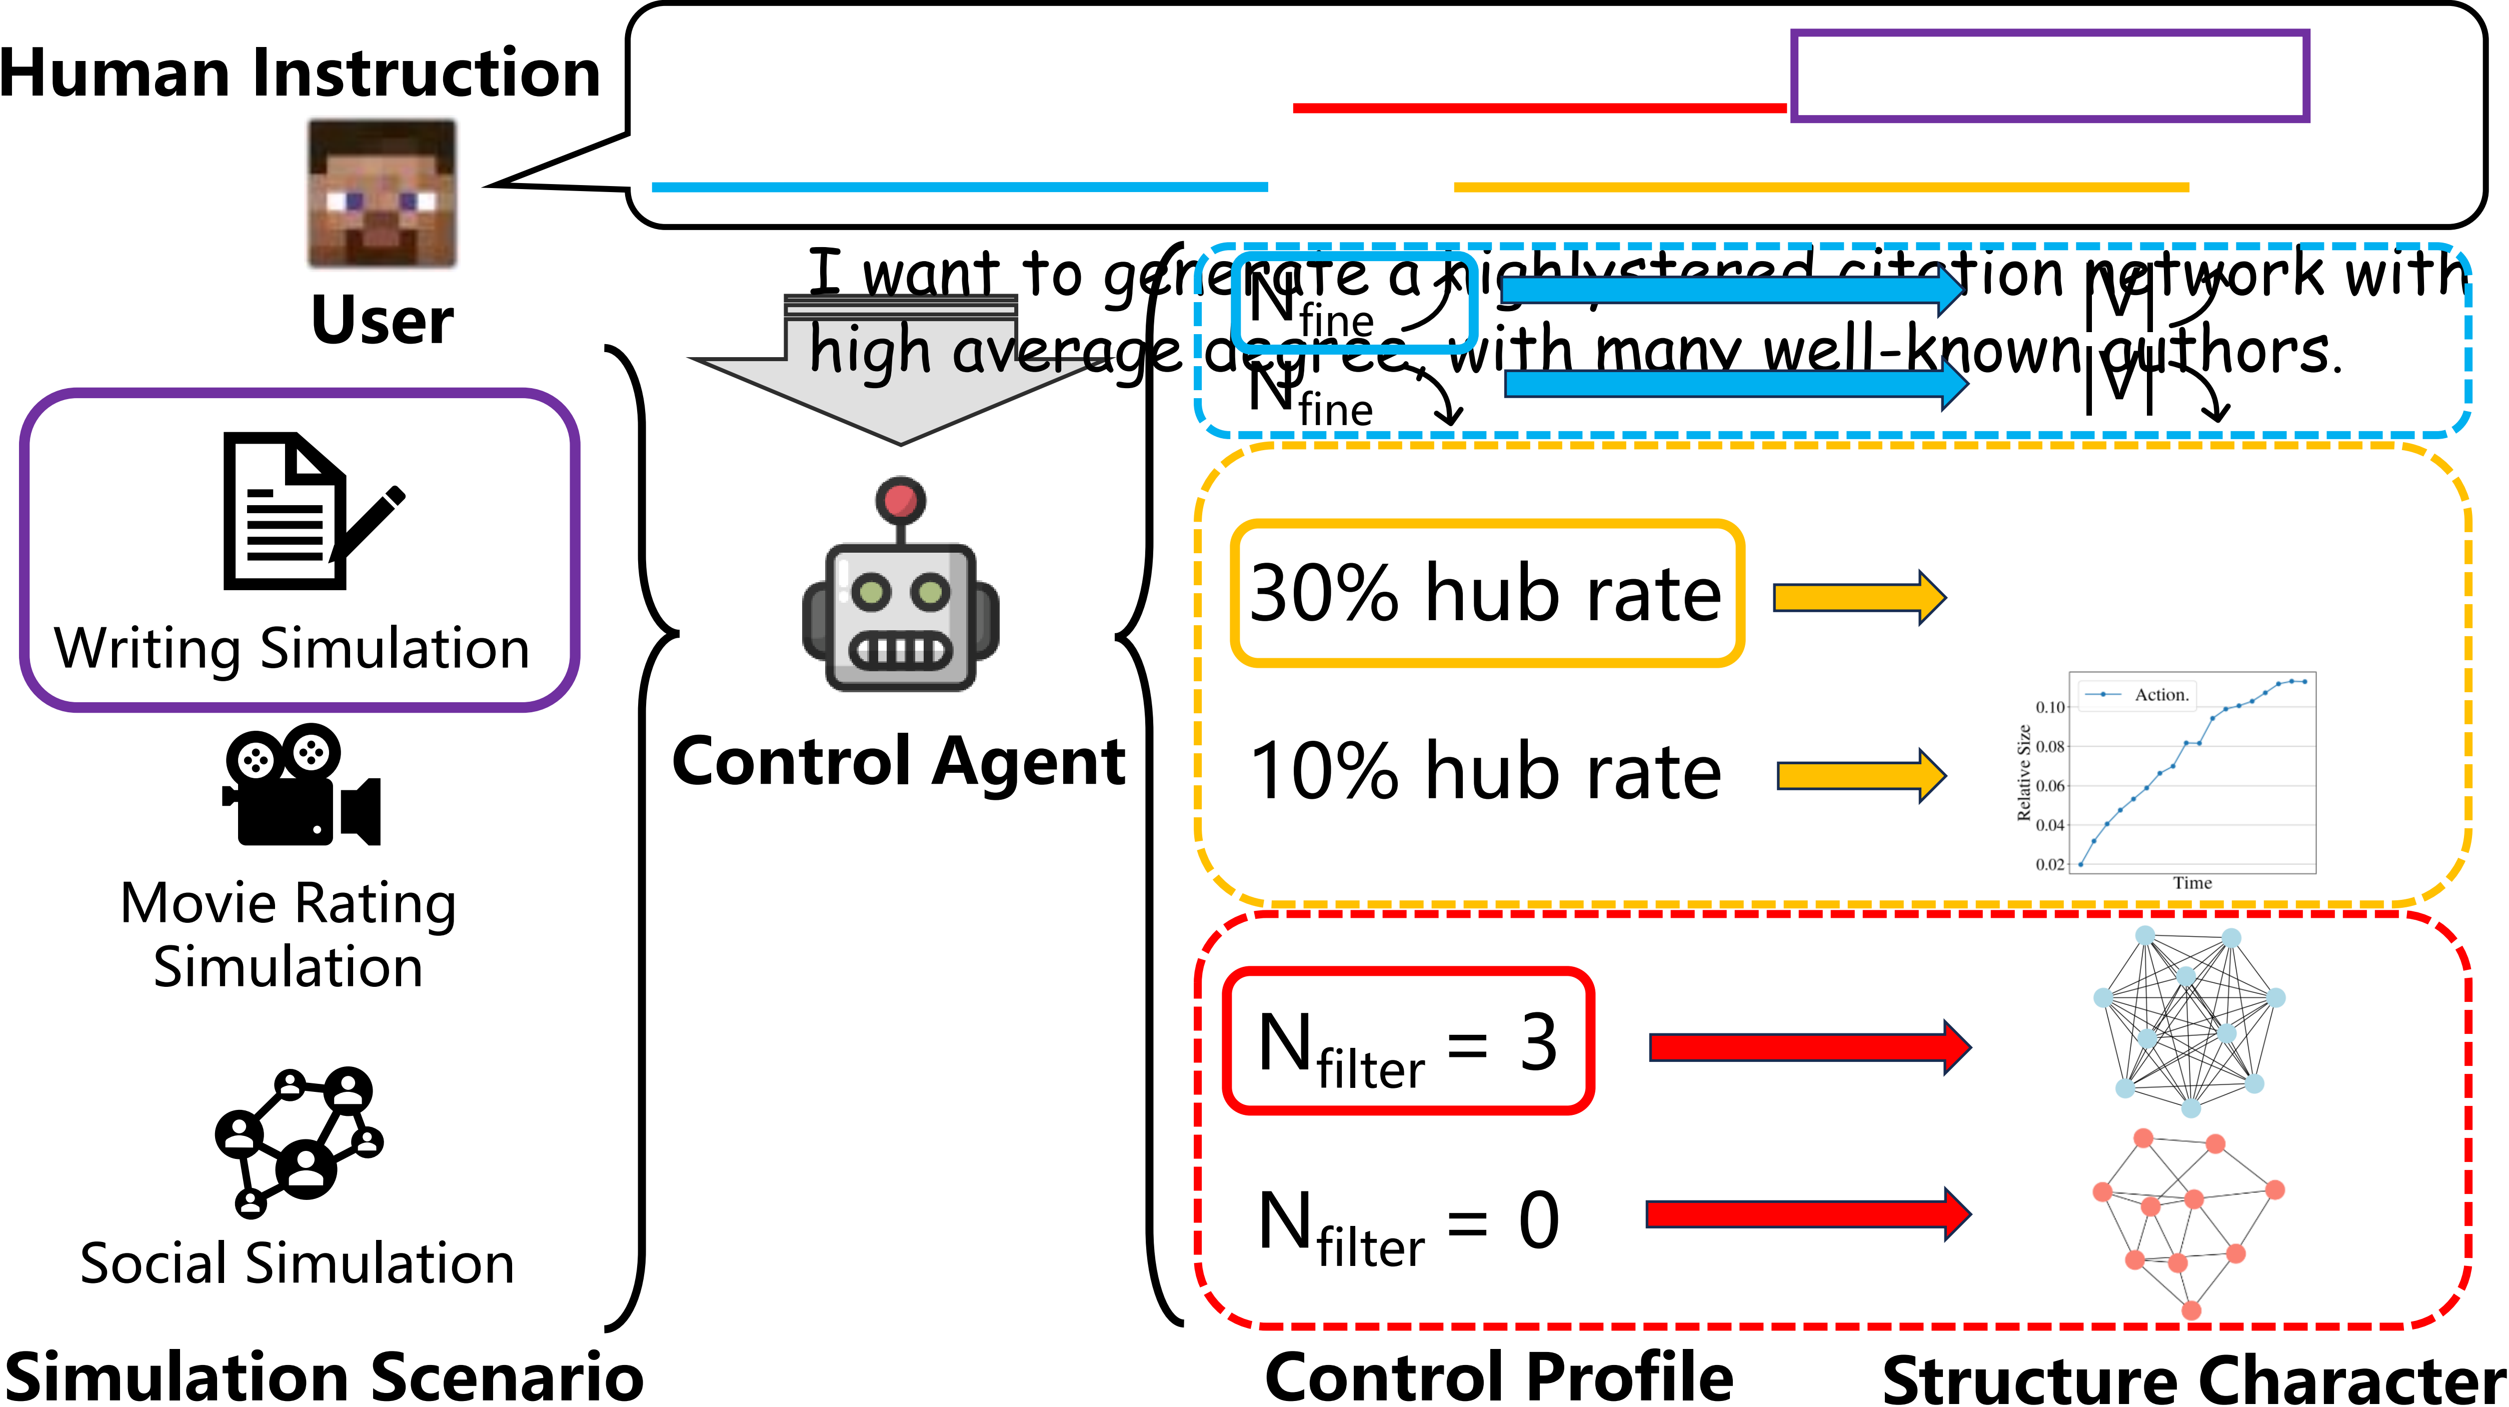
Human Instruction
User
high average degree, with many well-known authors.
Writing Simulation
Movie Rating Simulation
Social Simulation
Control Agent
N fine
|V|
30% hub rate
10% hub rate
Action.
Relative Size
Time
0.10
0.08
0.06
0.04
0.02
N filter = 3
N filter = 0
Simulation Scenario
Control Profile
Structure Character

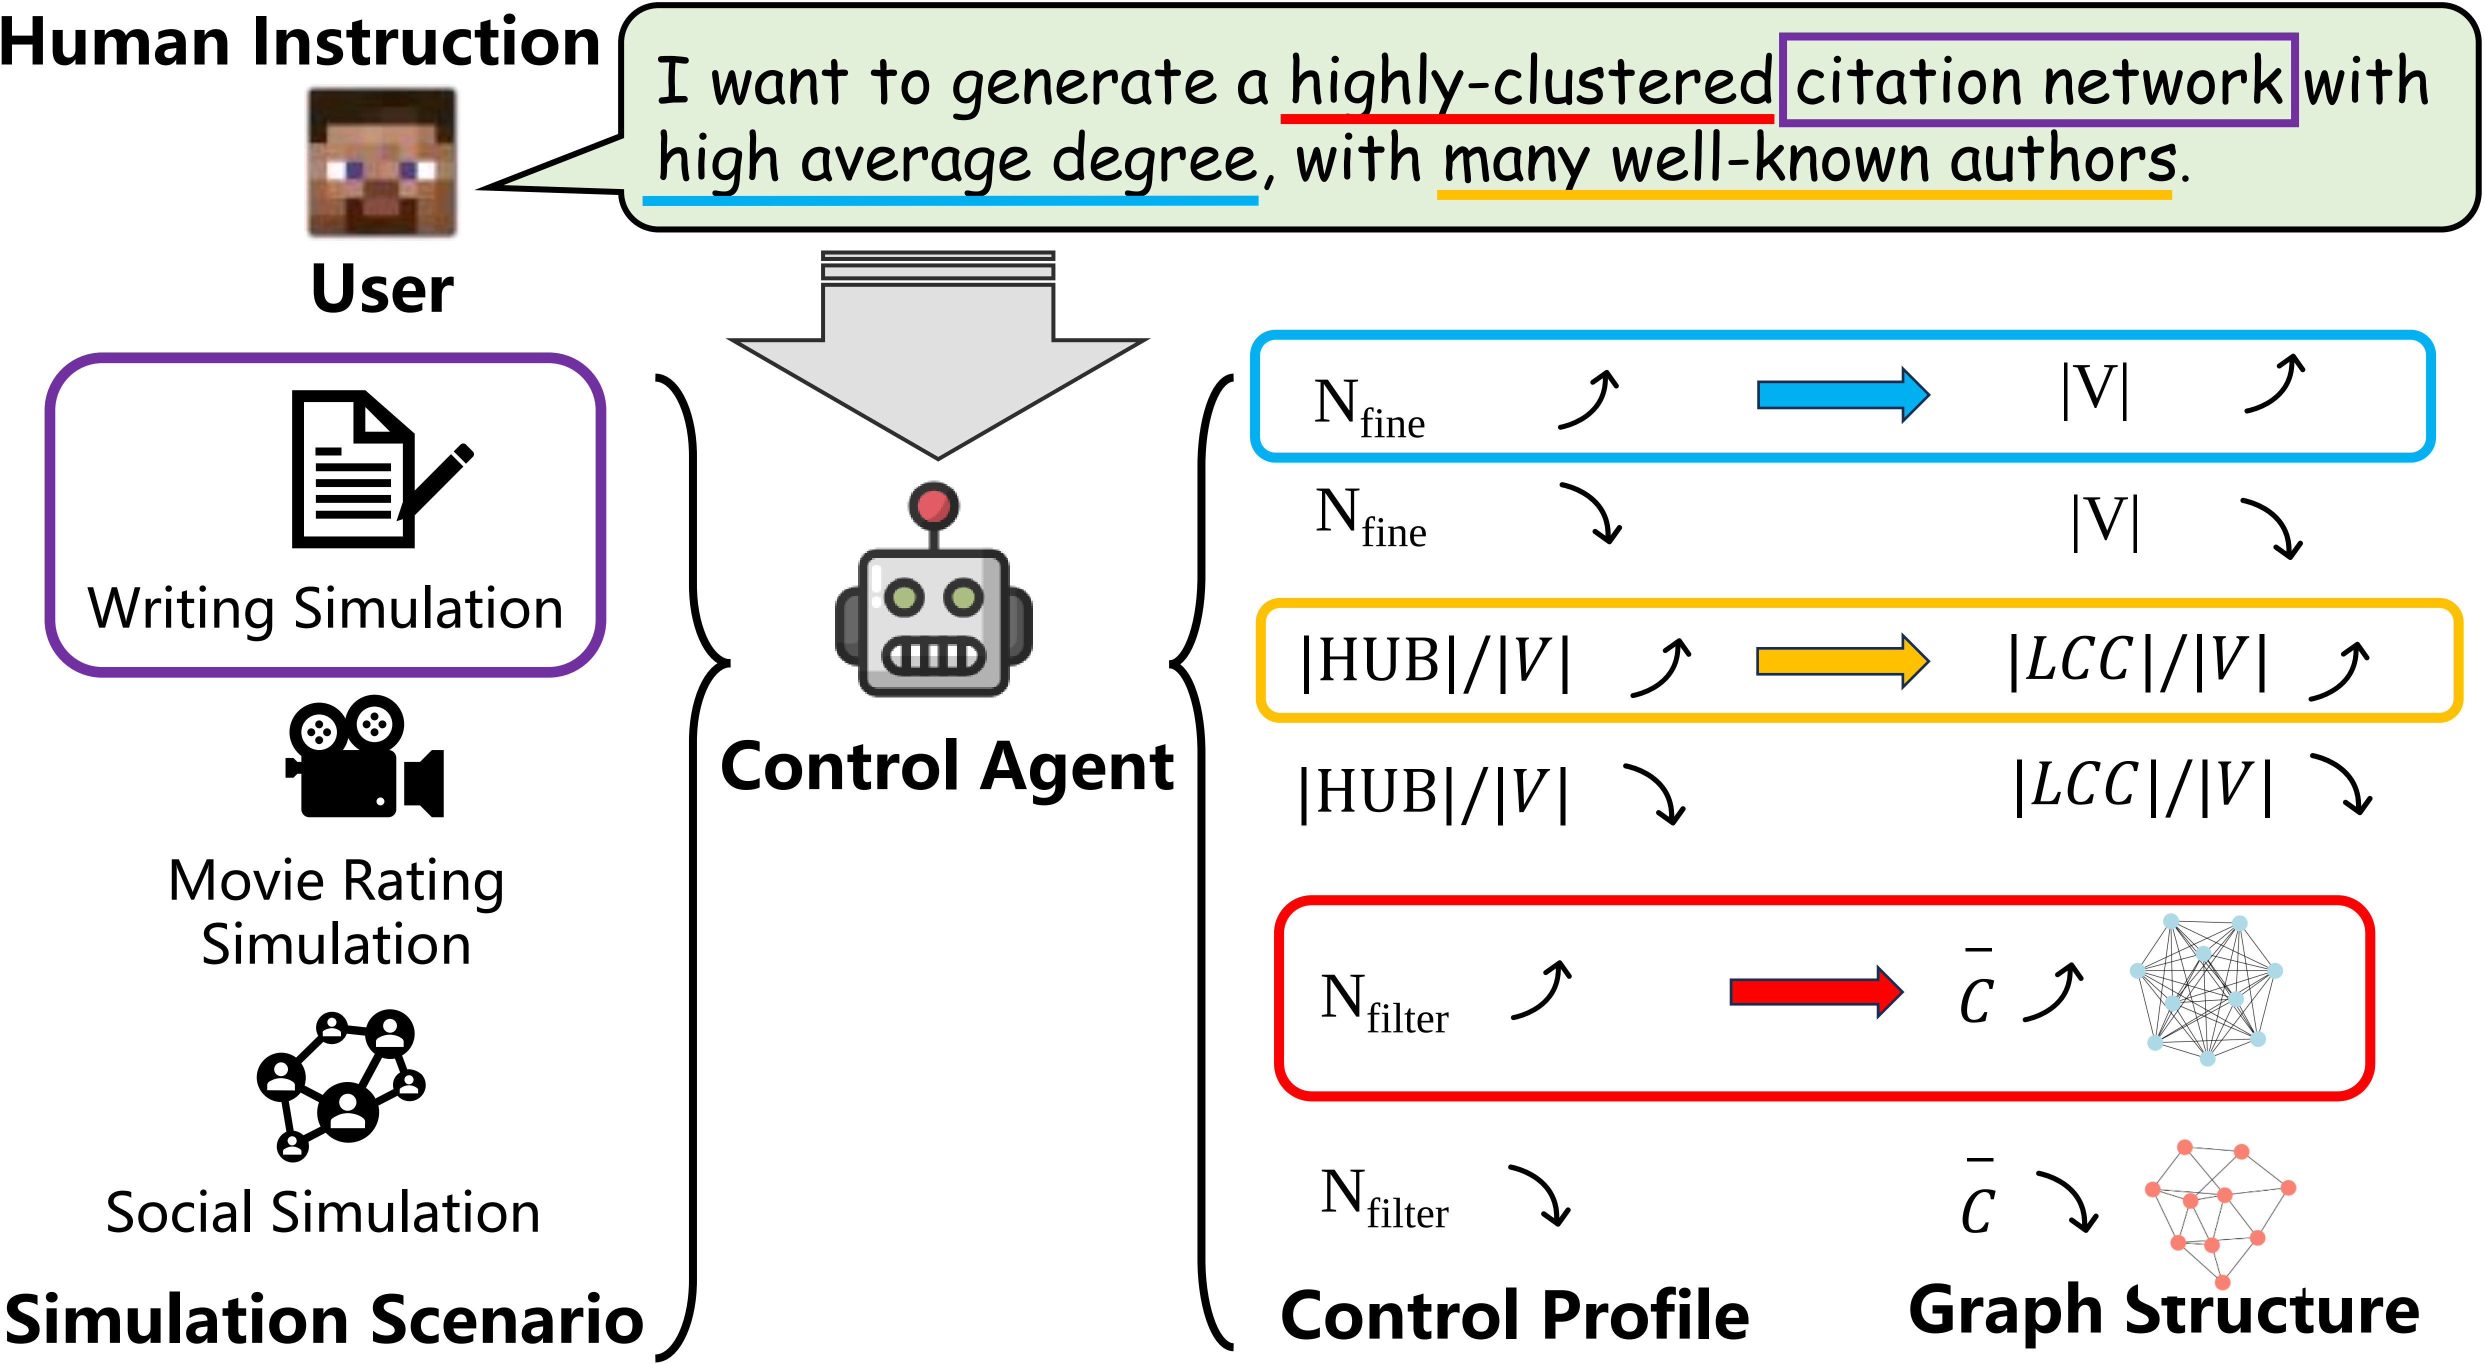

Human Instruction
I want to generate a highly-clustered citation network with high average degree, with many well-known authors.
User
Writing Simulation
Movie Rating Simulation
Social Simulation
Simulation Scenario
Control Agent
$N_{fine}$ ↗ |V| ↗
$N_{fine}$ ↘ |V| ↘
$|HUB|/|V|$ ↗ $|LCC|/|V|$ ↗
$|HUB|/|V|$ ↘ $|LCC|/|V|$ ↘
$N_{filter}$ ↗ $\bar{C}$ ↗
$N_{filter}$ ↘ $\bar{C}$ ↘
Control Profile
Graph Structure

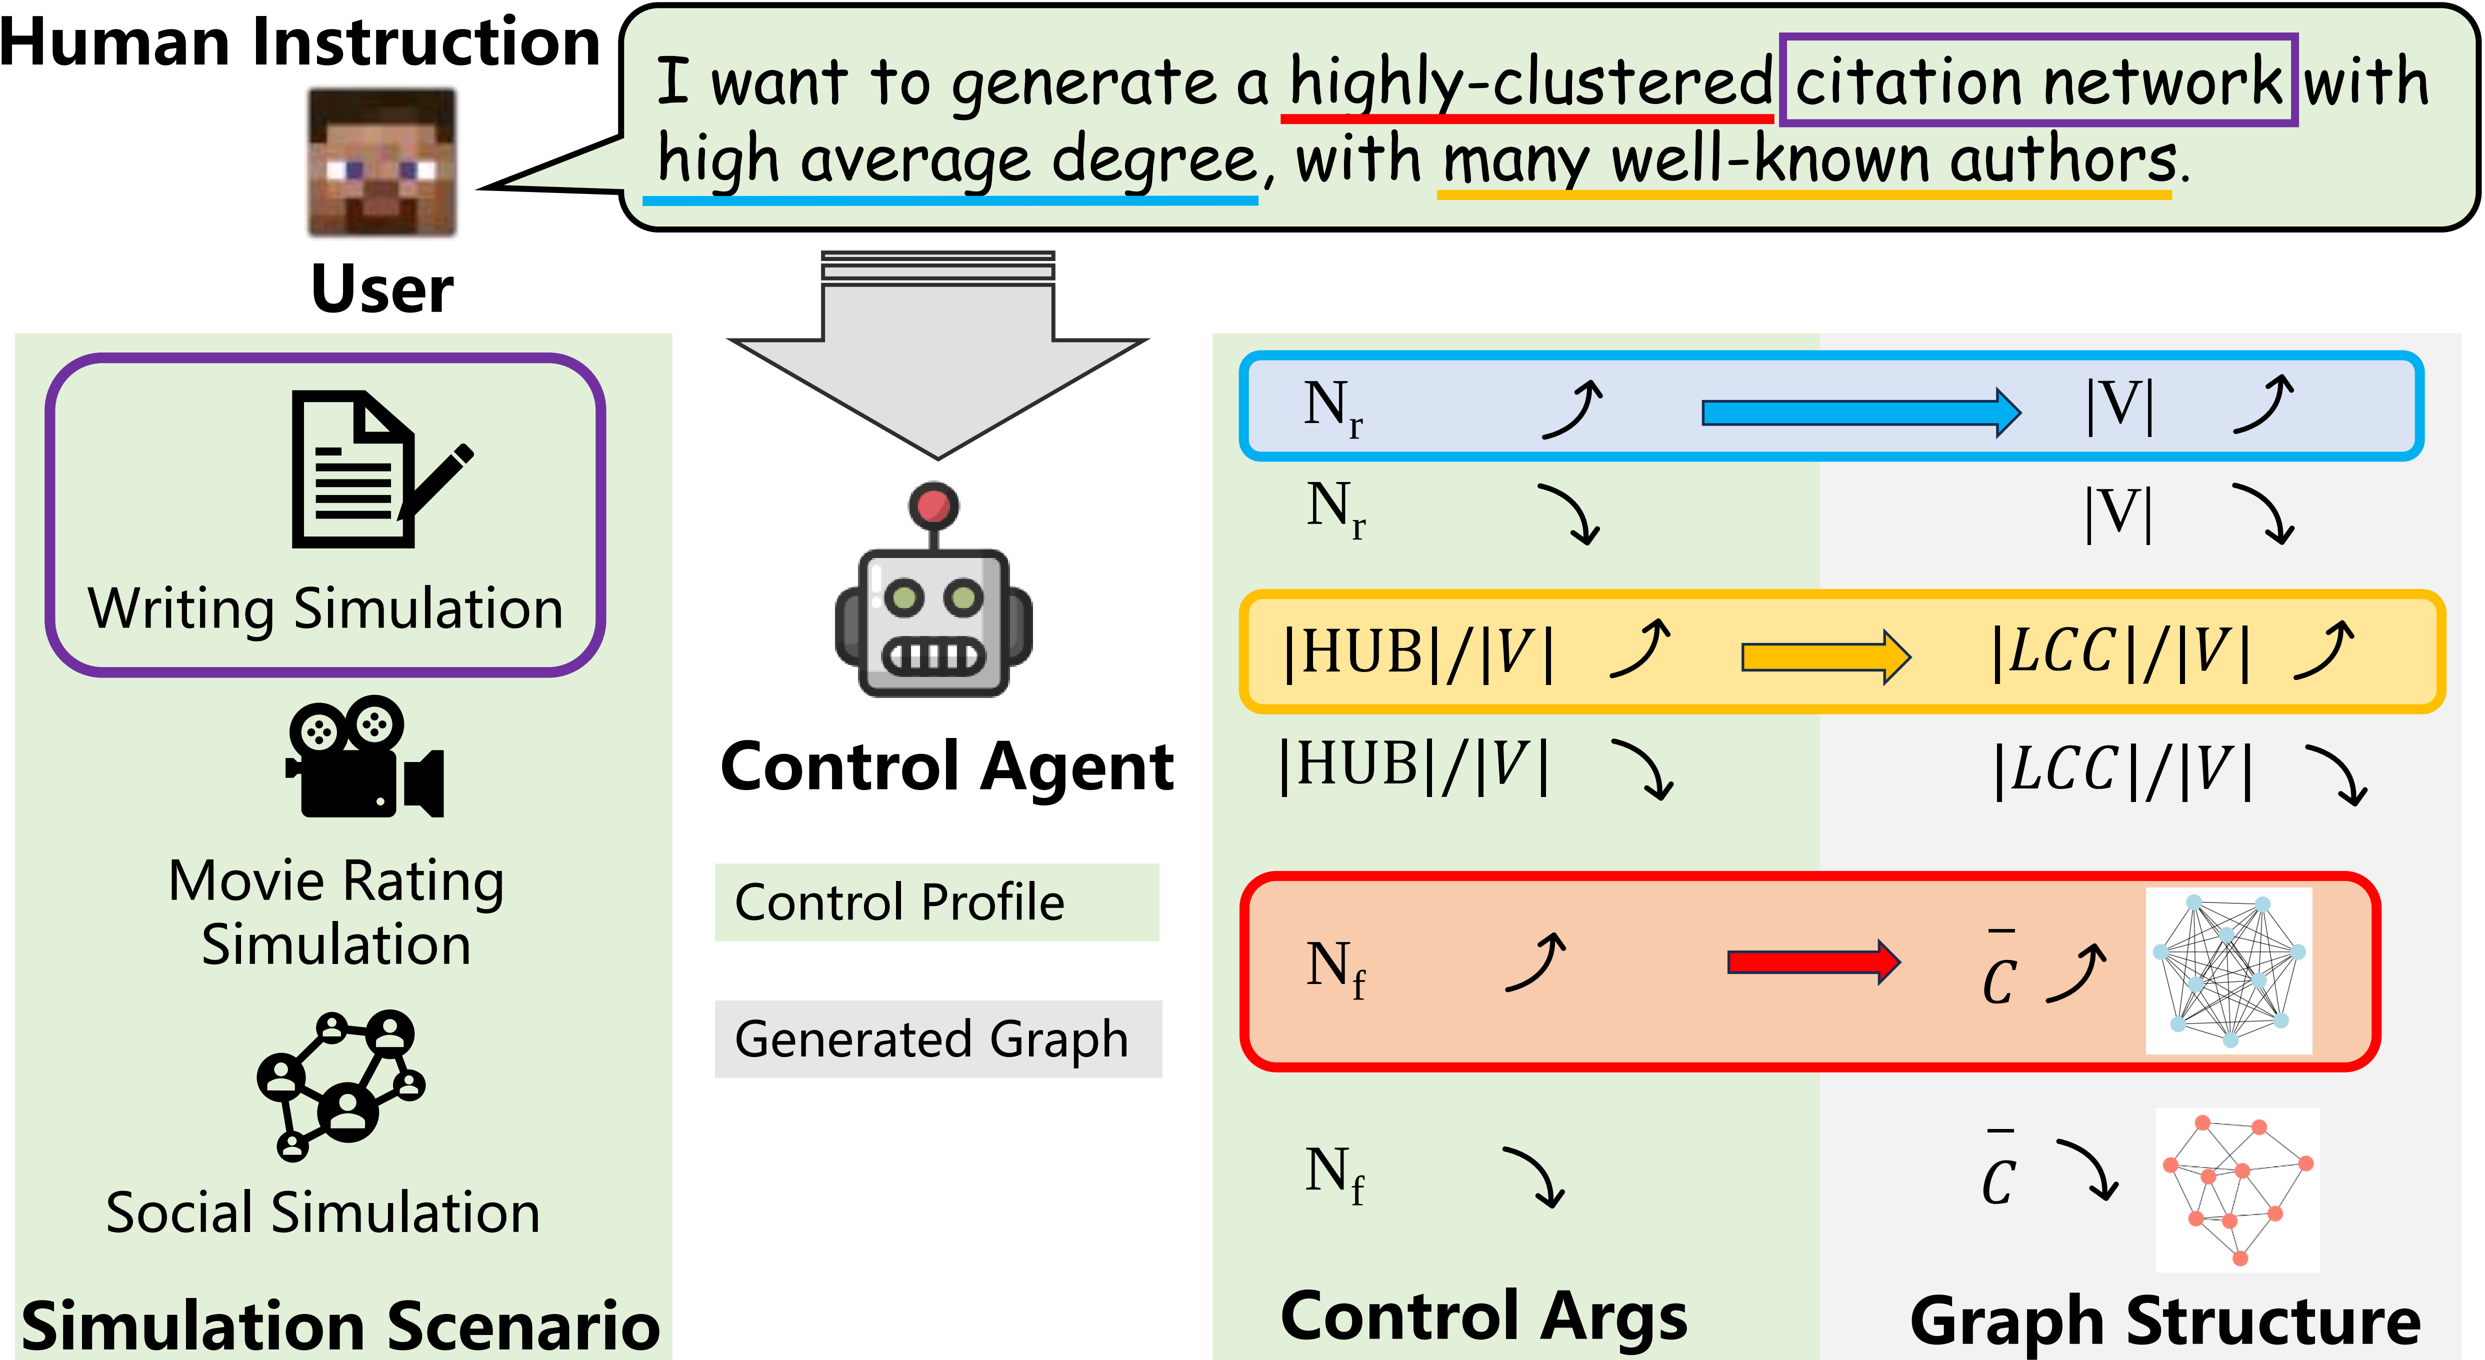

Human Instruction
I want to generate a highly-clustered citation network with high average degree, with many well-known authors.
User
Writing Simulation
Movie Rating Simulation
Social Simulation
Simulation Scenario
Control Agent
Control Profile
Generated Graph
N_r ↗ → |V| ↗
N_r ↘ |V| ↘
|HUB|/|V| ↗ → |LCC|/|V| ↗
|HUB|/|V| ↘ |LCC|/|V| ↘
N_f ↗ → C̄ ↗
N_f ↘ C̄ ↘
Control Args
Graph Structure

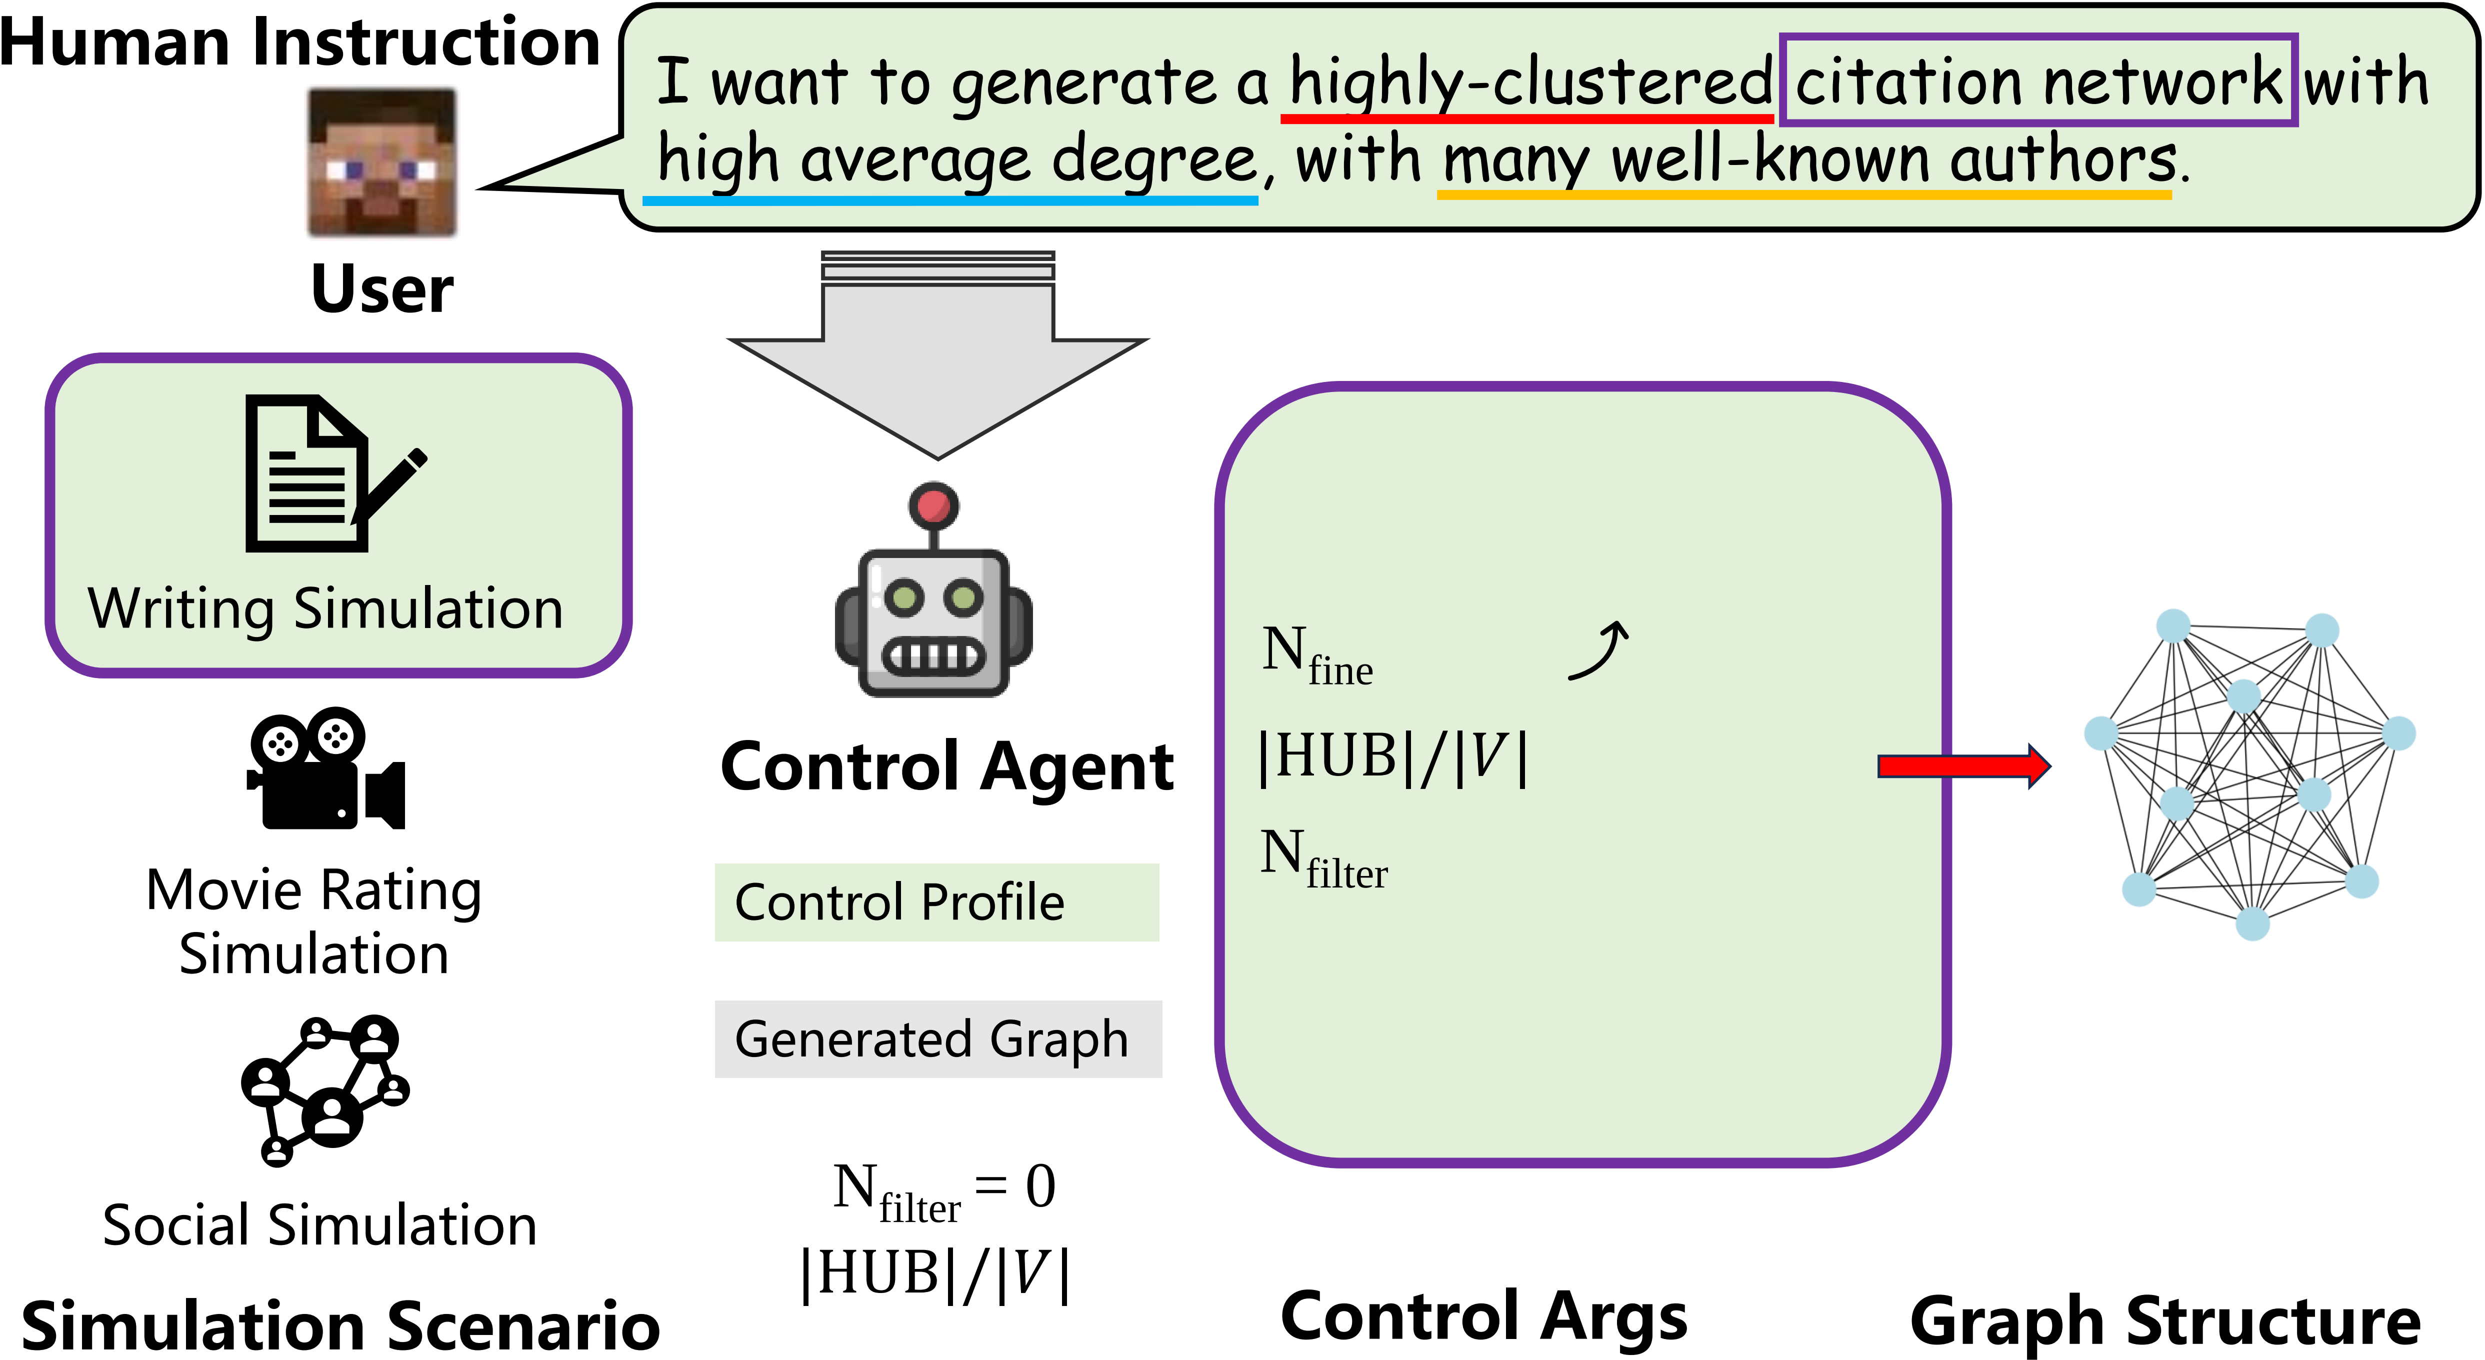
Human Instruction
I want to generate a highly-clustered citation network with high average degree, with many well-known authors.
User
Writing Simulation
Movie Rating Simulation
Social Simulation
Simulation Scenario
Control Agent
Control Profile
Generated Graph
$N_{filter} = 0$
$|HUB|/|V|$
$N_{fine}$
$|HUB|/|V|$
$N_{filter}$
Control Args
Graph Structure
