# Supplementary material for: LLM-Based Multi-Agent Systems are Scalable Graph Generative Models
Source: arXiv:2410.09824 source file (2025-01-06)
Supplement: Supplementary file 2 [file control.pdf]

# Human Instruction

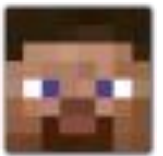

User

Writing Simulation

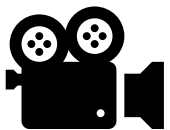

Movie Rating Simulation

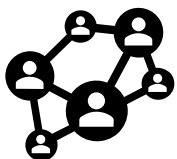

Social Simulation

Simulation Scenario

Control Agent

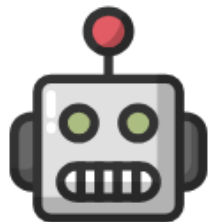

I want to generate a highly clustered citation network with high average degree, with many well-known authors.

30% hub rate

10% hub rate

$N_{\text{filter}} = 3$

$N_{\text{filter}} = 0$

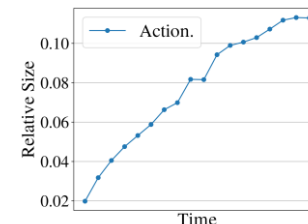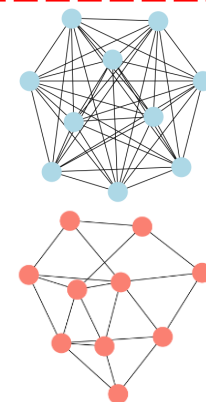

Control Profile

Structure Character

# Human Instruction

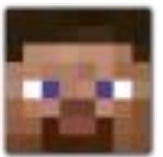

User

I want to generate a highly-clustered citation network with high average degree, with many well-known authors.

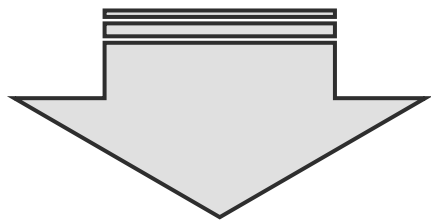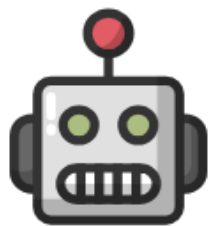

Control Agent

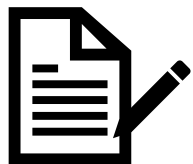

Writing Simulation

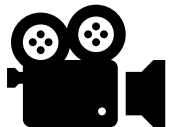

Movie Rating Simulation

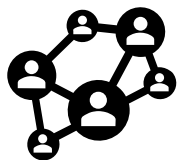

Social Simulation

Simulation Scenario

$N_{\text{fine}}$

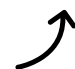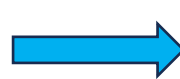

$|V|$

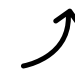

$N_{\text{fine}}$

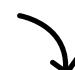

$|V|$

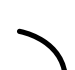

$|HUB|/|V|$

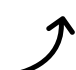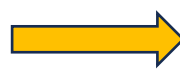

$|LCC|/|V|$

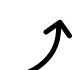

$|HUB|/|V|$

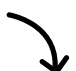

$|LCC|/|V|$

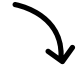

$N_{\text{filter}}$

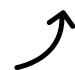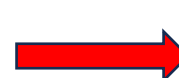

$\bar{C}$

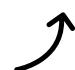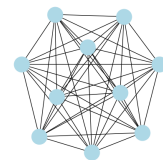

$N_{\text{filter}}$

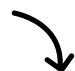

$\bar{C}$

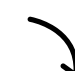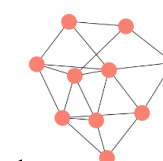

Control Profile

Graph Structure

# Human Instruction

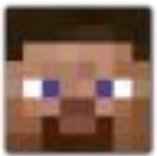

User

I want to generate a highly-clustered citation network with high average degree, with many well-known authors.

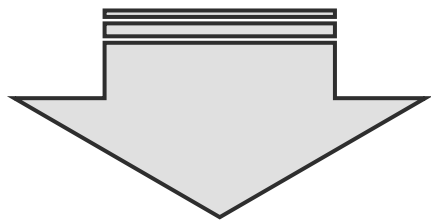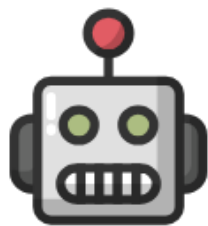

Control Agent

Control Profile

Generated Graph

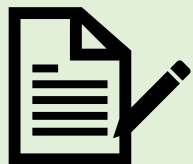

Writing Simulation

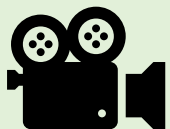

Movie Rating Simulation

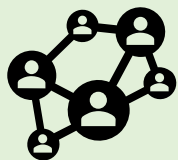

Social Simulation

Simulation Scenario

$N_r$

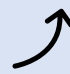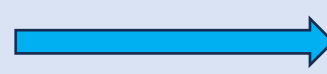

$|V|$

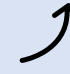

$N_r$

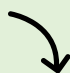

$|V|$

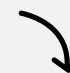

$|HUB|/|V|$

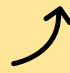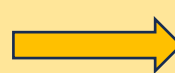

$|LCC|/|V|$

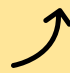

$|HUB|/|V|$

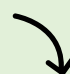

$|LCC|/|V|$

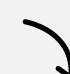

$N_f$

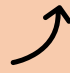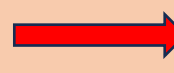

$\bar{c}$

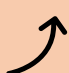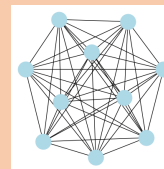

$N_f$

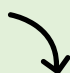

$\bar{c}$

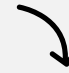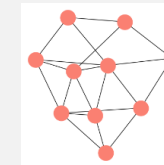

Control Args

Graph Structure

# Human Instruction

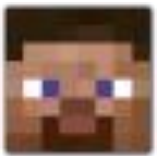

User

I want to generate a highly-clustered citation network with high average degree, with many well-known authors.

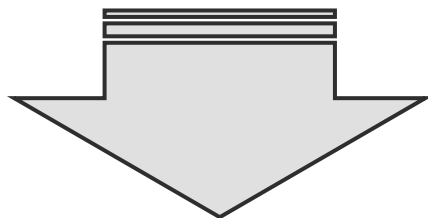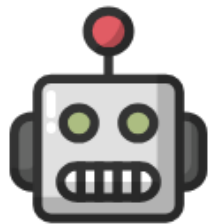

Control Agent

Control Profile

Generated Graph

$$N_{\text{filter}} = 0$$

$$|\text{HUB}|/|V|$$

$$N_{\text{fine}}$$

$$|\text{HUB}|/|V|$$

$$N_{\text{filter}}$$

Control Args

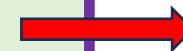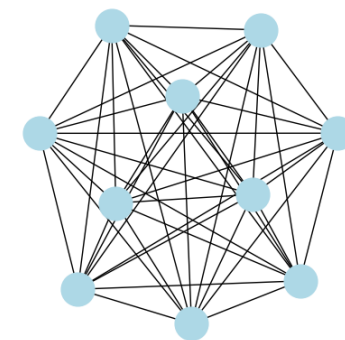

Graph Structure

Writing Simulation

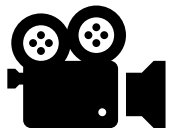

Movie Rating Simulation

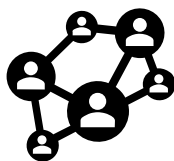

Social Simulation

Simulation Scenario
